# Supplementary material for: Coherent Acoustic Control of a Single Silicon Vacancy Spin in Diamond
Source: arXiv:1910.09710 ancillary file (2019-10-23)
Supplement: Supplementary file 1 [file saw-siv-supp.pdf]

# Supplementary Information for: Coherent Acoustic Control of a Single Silicon Vacancy Spin in Diamond

Smarak Maity,[1] Linbo Shao,[1] Stefan Bogdanović,[1] Srujan Meesala,[1] Young-Ik Sohn,[1] Neil Sinclair,[1,2]
Benjamin Pingault,[1] Michelle Chalupnik,[1] Cleaven Chia,[1] Lu Zheng,[3] Keji Lai,[3] and Marko Lončar[1,*]

[1] *John A. Paulson School of Engineering and Applied Sciences, Harvard University, 29 Oxford Street, Cambridge, MA 02138, USA*

[2] *Division of Physics, Mathematics and Astronomy, and Alliance for Quantum Technologies (AQT), California Institute of Technology, 1200 E. California Boulevard, Pasadena, CA 91125, USA*

[3] *Department of Physics, University of Texas at Austin, 110 Inner Campus Drive, Austin, TX 78705, USA*

* loncar@seas.harvard.edu

## I. COORDINATE SYSTEMS

We use $x, y, z$ to refer to the coordinate system of the devices. The axis normal to the diamond surface is denoted by $z$, which is the [001] lattice direction. The surface acoustic waves (SAWs) are launched along $x$, or the [110] lattice direction. The $y$ direction is given by the cross product of $z$ and $x$, and is along $[\bar{1}10]$.

The local coordinate system of the SiVs is referred to as $X, Y, Z$. The $C_3$ symmetry axis of the SiV, which is the line joining the two missing carbon atoms, is denoted by $Z$. This can be along any of the 4 equivalent $\langle 111 \rangle$ lattice directions. Because the SAWs are launched along [110], the 4 SiV axis directions are divided into two classes based on their orientation with respect to the [110] direction. "Longitudinal" SiVs have $Z$ along [111] or $[11\bar{1}]$, and "transverse" SiVs have $Z$ along $[1\bar{1}1]$ or $[\bar{1}11]$. The response of the two SiVs along both directions within each class is expected to be the same due to mirror symmetry of the SAWs about the $(\bar{1}10)$ plane. The $X$ and $Y$ directions are indicated in Fig. S1.

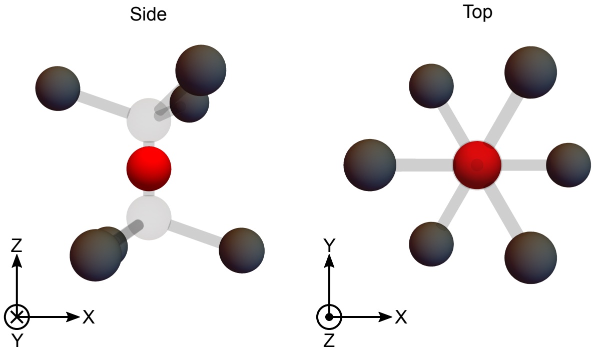


FIG. S1. Local coordinate system of the SiV.

## II. EXPERIMENTAL DETAILS

**Device fabrication.** We use [100]-cut, electronic grade single-crystal diamond samples synthesized by chemical vapor deposition (CVD) from Element Six Corporation. Silicon ions ($^{28}Si^{+}$) are implanted on the top surface of the diamond at an energy of 150 keV and a density of $10^{10}$cm$^{-2}$, introducing Si atoms over the entire surface at a depth of $100 \pm 18$ nm as determined by a SRIM simulation [S1]. SiV centers are generated by a high-temperature (1100° C), high-vacuum annealing procedure followed by a tri-acid clean (1:1:1 sulfuric, perchloric, and nitric acids). A 1.4 $\mu$m aluminum nitride (AlN) layer is deposited on top of the diamond by RF sputtering. SAW devices are fabricated using electron beam lithography followed by evaporation of 100 nm of gold (Au) for bonding pads and 75 nm of aluminum (Al) for IDTs.

**Electrical characterization of SAW devices.** These measurements are performed at room temperature. The IDTs are contacted with RF probes, which are connected to a vector network analyzer (Agilent E8364B) for $S$-parameter measurements.

**Microwave impedance microscopy measurements.** The IDT is driven by a continuous-wave microwave input signal to generate surface acoustic waves. An atomic force microscopy probe scans over the surface of the device and senses the electric potential at each point [S2, S3]. The measured signal is mixed with the drive signal to coherently detect the relative amplitude and phase of the electric potential of the SAWs.

**Low temperature experiments.** Low temperature experiments are performed in a closed-cycle liquid helium cryostat (Montana Instruments Cryostation). The sample is mounted on an XYZ piezoelectric nanopositioner stack (Attocube ANPx101 and ANPz101) with a custom-made holder. The holder contains another nanopositioner with a neodymium permanent magnet (K&J Magnetics) positioned behind the sample, that can be moved relative to the sample to adjust the magnetic field. The sample is clamped on top of the holder, using Indium foil for good thermal contact. A temperature sensor in the holder estimates the sample temperature to be about 5.8 K. A pair of IDTs are wire bonded to a PCB on the holder for electrical excitation and readout of acoustic pulses. SiVs in the sample are addressed with a home-built confocal microscope that focuses light from a 520 nm laser and a tunable 737 nm laser (M-Squared SolSTiS) on the sample. The 520 nm laser is periodically switched on to reset the charge state of the SiV, while the 737 nm laser is used to resonantly excite optical transitions. The wavelength of the tunable laser is

stabilized by using feedback from a wavemeter (HighFinesse WS7). Photons emitted by the SiV in the phonon side band (PSB) > 740 nm are selected by an optical long-wavelength pass filter and sent to an avalanche photo diode (APD, Excelitas) for counting.

**Pulsed measurements of SiVs.** Laser pulses at 737 nm are generated with an electro-optic intensity modulator (EOM, iXblue NIR-MX800). The EOM is biased at its half-wave voltage ($V_\pi$) and stabilized against temporal drift by using feedback with a lock-in amplifier (SRS SR830). A delay generator (SRS DG645) is used to generate the voltage pulses sent to the EOM. Acoustic pulses are produced by exciting the SAW transducers with short microwave pulses, which are generated with an arbitrary waveform generator (AWG, Tektronix AWG70001A) and amplified with an RF amplifier (Pasternack PE15A3008). The AWG clock is synchronized to the delay generator to prevent clock skew. Optical and acoustic pulses are temporally aligned by adjusting the delay of the waveform on the AWG.

## III. TIME DOMAIN CHARACTERIZATION OF SAW DEVICES

To perform time-domain characterization, half of the electrical input to the device is sent to a real-time oscilloscope (Tektronix MSO71604C) by way of a 50-50 RF power splitter. One of the IDTs in a pair is excited with the AWG, and the signal from the other IDT is also connected to the oscilloscope. Short electrical pulses are generated with the AWG and both the AWG pulse and the transmitted electrical pulse from the SAW are characterized (Fig. S2). The ringing of the input signal is caused by the RF amplifier. The transmitted output signal has two main features:

1. The earliest feature is due to direct electrical crosstalk between the input and output ports. It has approximately the same length as the input pulse. This is likely from the wire bonds to the input and output transducers, because these GHz-frequency electrical signals have a relatively large wavelength in air. The delay between the input signal and the crosstalk signal is due to the longer path via RF cables to the device inside the cryostat and back.

2. Next, there is the feature from the transduced SAW pulse. This ramps up and down, indicating the build-up and decay of the acoustic pulse that is expected from the non-zero length of the transducer.

The delay between the electrical crosstalk and the first acoustic response indicates a time of about 21 ns for the SAW pulse to travel between the transducers. Given that the separation between the transducers is approximately 175 $\mu$m, the SAW velocity is approximately 8.3 km/s which agrees with simulations. The non-zero length of the SAW transducer imposes a lower bound on the shortest acoustic pulses it can generate, which is about 13 ns. As the length of the microwave pulse from the AWG is increased, the length of the acoustic pulse remains approximately constant while its amplitude increases. For pulses longer than 13 ns, the acoustic pulse reaches its maximum amplitude and its length starts to increase, as expected.

Because of the minimum duration of the SAW pulses, we use a minimum delay of 10 ns between $\pi/2$ pulses for the Ramsey interferometry measurement. At this delay, the acoustic pulses overlap neglegibly (Fig. S3).

## IV. CALIBRATION OF OPTICAL AND ACOUSTIC PULSE TIMING

The fluorescence intensity from an SiV under optical excitation can vary in the presence of an acoustic pulse. This is observed when the laser frequency is resonant with a transition to a virtual state generated by the acoustic pulse, as explained in Section VII. We explore this interaction by performing pulsed measurements of an SiV under a magnetic field, using different frequencies of optical and acoustic pulses, as shown in Fig. S4. The SiV spin is initialized and read out using laser pulses, similar to the experiments in the main text, and an acoustic pulse is applied during the initialization pulse. In (a), the laser is detuned by $f = 3.34$ GHz from the C3 transition, and the SAW frequency is set to the detuning $f$. The laser frequency is not resonant with any of the other transitions. Hence we notice very low fluorescence intensity during the optical pulse, but there is a large increase in counts when the acoustic pulse is applied, due to the photon-phonon transition being resonant with C3. In (b), the laser is resonant with the C1 transition, and the SAW frequency is set to the difference between the C1 and C3 transitions, equivalent to the splitting between the lower ground states $|e_{g+} \downarrow\rangle$ and $|e_{g-} \uparrow\rangle$ of the SiV. There is an initial increase in the fluorescence due to the optical pulse, followed by the exponential decay as the spin population is optically pumped to $|e_{g-} \uparrow\rangle$. When the acoustic pulse is applied, the photon-phonon transition is resonant with C3, thereby leading to a large increase of fluorescence.

This response has practical significance for our experiment, as it allows the identification of the time of arrival of the acoustic pulse at the SiV. This is used to measure the velocity of the acoustic pulse on the diamond surface, and to establish that it is indeed the acoustic pulse that is responsible for controlling the SiV spin. To do this, we choose

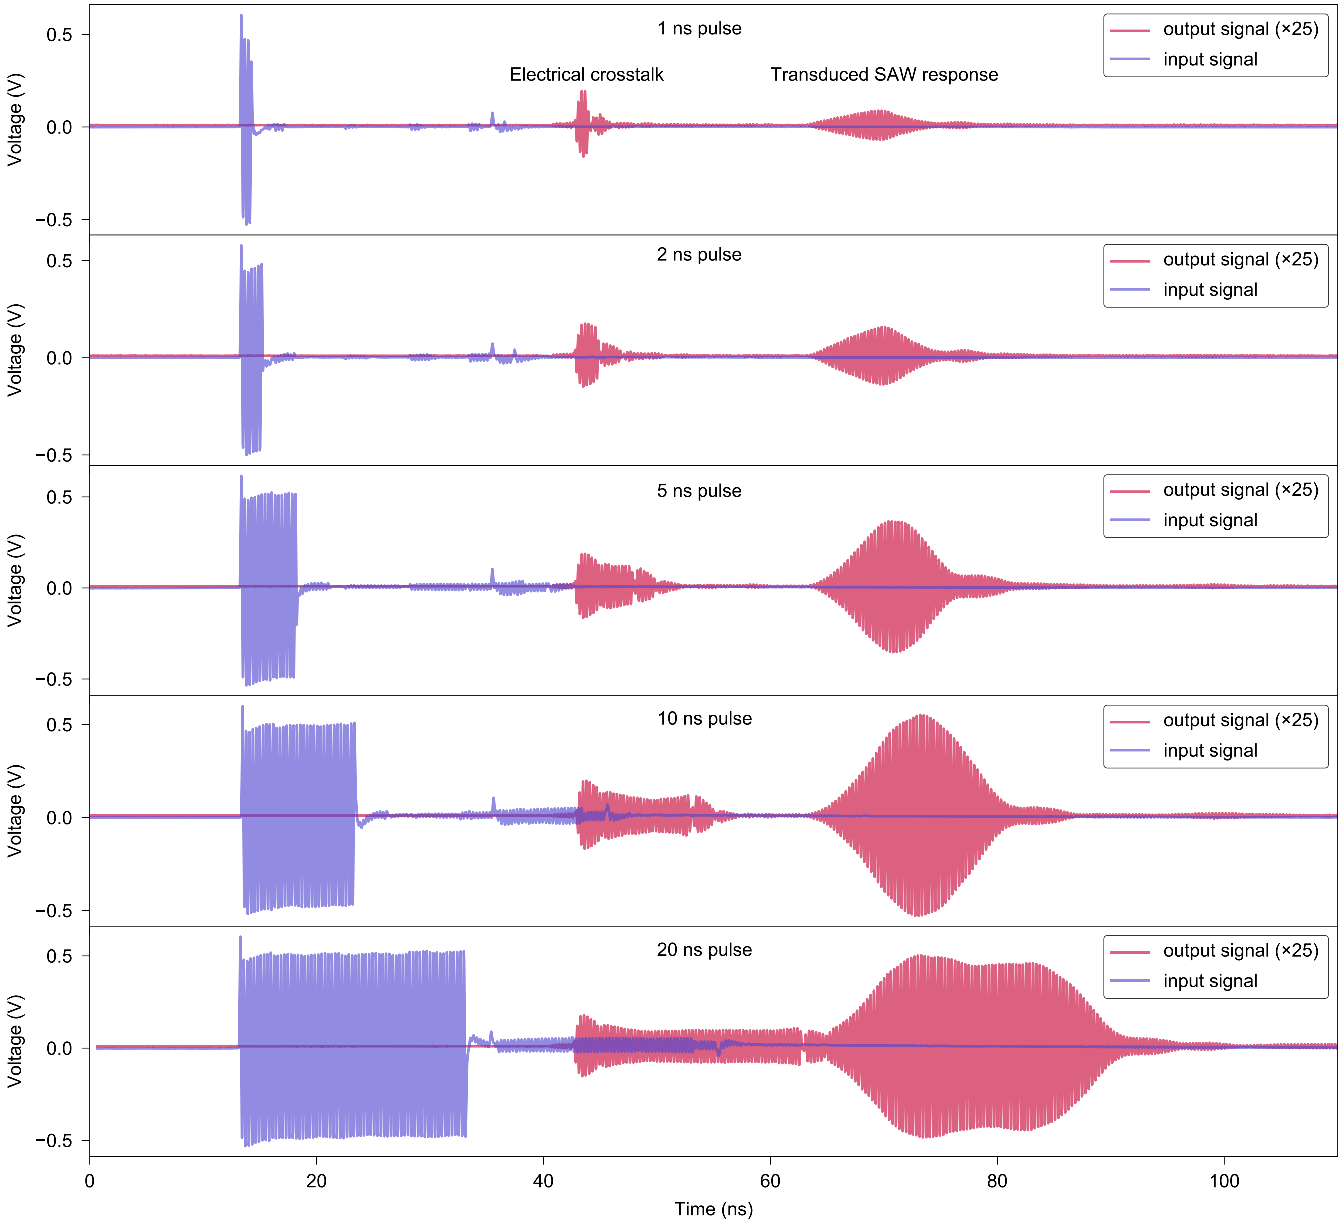


FIG. S2. Time domain characterization of SAW devices with short electrical pulses. The frequency of the pulses was set to 3.37 GHz for optimal transducer response.

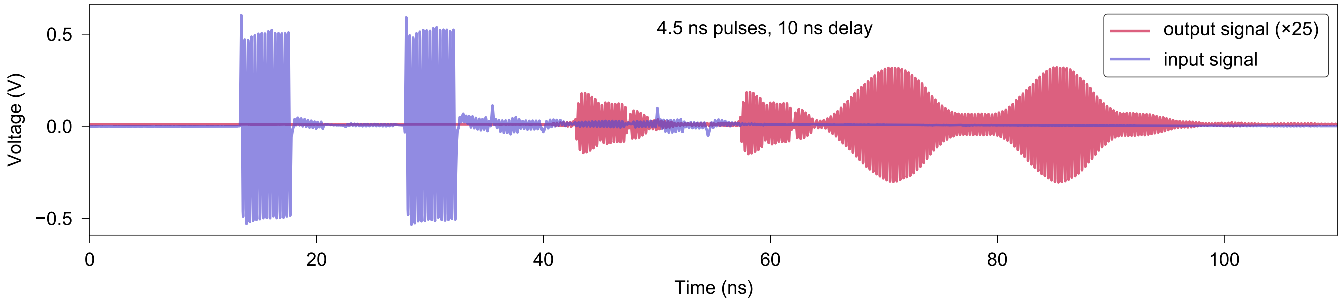


FIG. S3. Time domain chracterization of SAW devices using two 3.38 GHz, 4.5 ns $\pi/2$ pulses separated by 10 ns.

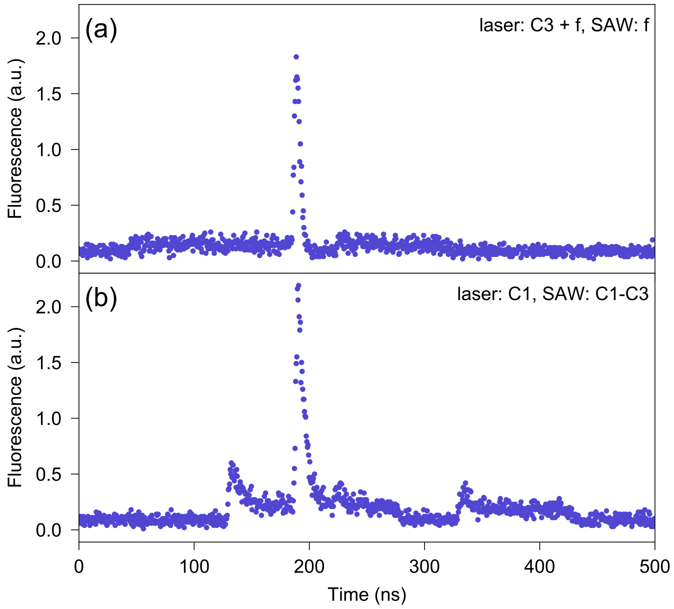


FIG. S4. Pulsed optical and acoustic measurements demonstrating $A_{1g}$ strain response of the SiV.

a different SiV, one located close (∼ few $\mu$m) to one of the transducers (i.e. the "right" transducer). We repeat the measurement from Fig. S4(b), first generating the acoustic pulse by exciting the right transducer. Then we swap the RF cables connected to the IDTs, in order to switch the roles of the left and right transducers. We repeat the measurement, this time by exciting the left transducer. The resulting time-resolved fluorescence (Fig. S5) indicates a time difference of about 13.3 ns between the arrival of the acoustic pulses from the right and left at the SiV. Because we swap the RF cables for the second measurement, the time difference from different lengths of RF cables to the left and right ports of the cryostat is eliminated. There is still a small difference in the lengths of the wires inside the cryostat, however this difference is on the order of a few cm and is thus neglegible. Therefore the measured time difference is close to the time taken for the SAW pulse to travel between the left and right transducer. Given that the separation between transducers is 175 $\mu$m, we estimate a velocity of 13.1 km/s for the SAW. While the estimate of the SAW velocity from the SiV fluorescence measurement and electrical measurements differ, they are both close (within 25%) of the simulated value (10.3 km/s). This indicates that these are indeed acoustic pulses driving the SiV, and not microwave radiation that might originate from the patterned electrodes (e.g. the IDTs).

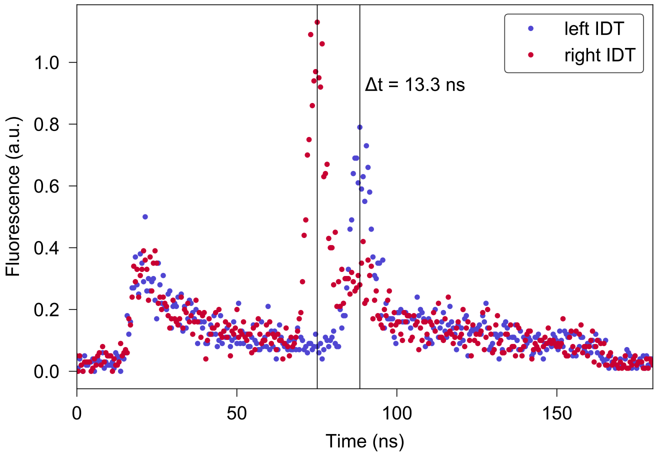


FIG. S5. Measurement of SAW velocity using SiV fluorescence.

## V. FITTING OF RABI OSCILLATION DATA

As mentioned in the main text, we use a simple two-level model (exponentially damped sinusoid) to fit the Rabi oscillation data. This model fits the data fairly well for low acoustic powers, but begins to show deviations at higher powers (Fig. S6). Fitting the data using a master equation model which considers all 4 levels in the SiV ground state, similar to the approach in [S4], does not provide any significant improvement over the simple model. We believe that the distortions in the oscillations may be due to reflections of the acoustic pulses from the opposing IDTs. Fabrication of IDTs individually, instead of in pairs, may provide an answer to this question.

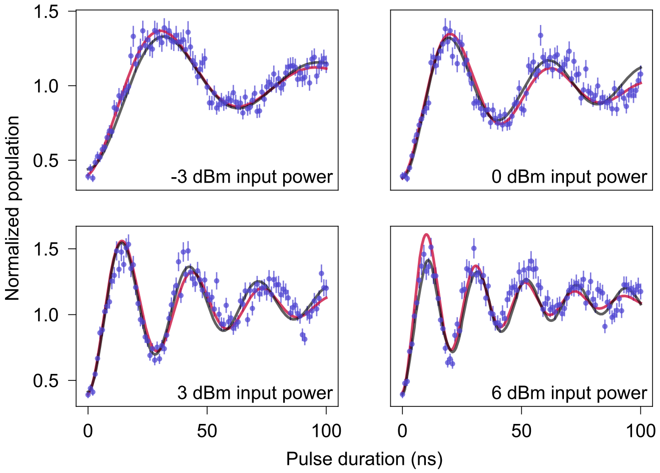


FIG. S6. Rabi oscillation measurement data for all 4 input powers. The red and black curves show the results of the two-level model and the four-level master equation model, respectively.

## VI. SIV HAMILTONIAN

The SiV has four states in both the ground and excited state manifolds, given by the direct product of the orbital $\{|e_X\rangle, |e_Y\rangle\}$ and spin $\{|\uparrow\rangle, |\downarrow\rangle\}$ bases. For the purposes of our experiments, the SiV Hamiltonian can be expressed as a sum of spin-orbit, Zeeman, and strain terms [S5, S6]. The constants appearing in these expressions have two sets of values for the ground and excited states. The spin-orbit term is given by

$$\mathcal{H}_{\mathrm{SO}} = -\frac{\lambda_{\mathrm{SO}}}{2} L_Z S_Z \tag{S1}$$

$$= -\frac{\lambda_{\mathrm{SO}}}{2} \begin{bmatrix} 0 & i \\ -i & 0 \end{bmatrix} \otimes \begin{bmatrix} 1 & 0 \\ 0 & -1 \end{bmatrix} \tag{S2}$$

in which $\lambda_{\mathrm{SO}}$ is the spin-orbit coupling. The Zeeman term is given by

$$\mathcal{H}_{\mathrm{Z}} = q\gamma_L L_Z B_Z + \gamma_S \vec{S} \cdot \vec{B} \tag{S3}$$

$$= q\gamma_L B_Z \begin{bmatrix} 0 & i \\ -i & 0 \end{bmatrix} \otimes \mathcal{I}_2 \tag{S4}$$

$$+ \frac{\gamma_S}{2} \mathcal{I}_2 \otimes \begin{bmatrix} B_Z & B_X - iB_Y \\ B_X + iB_Y & -B_Z \end{bmatrix} \tag{S5}$$

in which $\gamma_L = \mu_B/\hbar, \gamma_S = 2\mu_B/\hbar$ are the orbital and spin gyromagnetic ratiosrespectively, and $q$ is the orbital quenching factor. The strain Hamiltonian is given by

$$\mathcal{H}_{\mathrm{strain}} = \begin{bmatrix} \alpha - \beta & \gamma \\ \gamma & \alpha + \beta \end{bmatrix} \otimes \mathcal{I}_2 \tag{S6}$$

| Constant | Value | Unit | Reference |
|---|---|---|---|
| $\lambda_{\mathrm{SO},g}$ | 45 | GHz | [S5] |
| $\lambda_{\mathrm{SO},e}$ | 257 | GHz | [S5] |
| $\gamma_S$ | 28 | GHz/T | [S5] |
| $\gamma_L$ | 14 | GHz/T | [S5] |
| $q$ | 0.1 | 1 | [S5] |
| $t_{\parallel,e} - t_{\parallel,g}$ | -1.7 | PHz/strain | [S6] |
| $t_{\perp,e} - t_{\perp,g}$ | 0.078 | PHz/strain | [S6] |
| $d_g$ | 1.3 | PHz/strain | [S6] |
| $d_e$ | 1.8 | PHz/strain | [S6] |
| $f_g$ | -1.7 | PHz/strain | [S6] |
| $f_e$ | -3.4 | PHz/strain | [S6] |

TABLE I. Measured constants of the SiV Hamiltonian

in which $\alpha, \beta, \gamma$ are symmetry-adjusted linear combinations of strain tensor components and are given by

$$\alpha = t_\perp(\epsilon_{XX} + \epsilon_{YY}) + t_\parallel \epsilon_{ZZ}, \tag{S7}$$

$$\beta = d(\epsilon_{XX} - \epsilon_{YY}) + f\epsilon_{ZX}, \tag{S8}$$

$$\gamma = -2d\epsilon_{XY} + f\epsilon_{YZ}. \tag{S9}$$

Hence $\alpha$ consists of strain components belonging to the $A_{1g}$ representation of the $D_{3d}$ symmetry group and $\beta, \gamma$ consist of the $E_{gX}, E_{gY}$ representation components. The measured values of the constants associated with each of the terms in the Hamiltonian have been reported previously and are summarized in Table I.

## VII. STRAIN RESPONSE OF THE SIV

In the coordinate system of the devices (Fig. 2(a) of the main text), the SAW mostly has components in the $x$ and $z$ directions, with $x$ being the direction of propagation. Hence the components of the strain involving $y$ can be neglected. From our simulations, we notice that the components $\epsilon_{xx}$ and $\epsilon_{zz}$ are in phase while $\epsilon_{xz}$ is $\pi/2$ out of phase. Hence the strain tensor of the SAW in device coordinates may be expressed as

$$\epsilon_{\mathrm{device}} = \begin{bmatrix} \epsilon_{xx} & 0 & -i\epsilon_{xz} \\ 0 & 0 & 0 \\ -i\epsilon_{xz} & 0 & \epsilon_{zz} \end{bmatrix}. \tag{S10}$$

The SiV responds differently to strain components belonging to the $A_{1g}$ and $E_g$ representations. The $A_{1g}$ strain components $\epsilon_{ZZ}$ and $\epsilon_{XX} + \epsilon_{YY}$ (in SiV coordinates) shift the energies of the SiV electronic states, while the $E_g$ strain components $\epsilon_{XX} - \epsilon_{YY}$, $\epsilon_{XZ}$, $\epsilon_{XY}$ and $\epsilon_{YZ}$ mix the electronic orbitals [S6]. While the $E_g$ strain response is responsible for the acoustic spin control, the $A_{1g}$ response is also of practical significance to this experiment, as mentioned in Section IV.

### A. $A_{1g}$ strain response

When the SiV is subjected to an oscillating $A_{1g}$ strain field, the oscillating energy shift of the electronic states causes frequency modulation of the energy levels, generating virtual states from interaction with an integer number of phonons. These virtual states are revealed as sidebands in the resonant excitation spectrum under continuous-wave acoustic driving (Fig. S7). As the acoustic power is increased, more sidebands are observed. We observe two sidebands using 6 dBm of microwave input power applied to the transducer, demonstrating photon-phonon transitions with up to two phonons.

Since these measurements are performed at zero magnetic field, the SiV can be described by just the spin-orbit and strain Hamiltonian terms:

$$\mathcal{H} = \mathcal{H}_{\mathrm{SO}} + \mathcal{H}_{\mathrm{strain}} \tag{S11}$$

$$= -\frac{\lambda_{\mathrm{SO}}}{2}\begin{bmatrix} 0 & i \\ -i & 0 \end{bmatrix} \otimes \begin{bmatrix} 1 & 0 \\ 0 & -1 \end{bmatrix} + \begin{bmatrix} \alpha - \beta & \gamma \\ \gamma & \alpha + \beta \end{bmatrix} \otimes \mathcal{I}_2 \tag{S12}$$

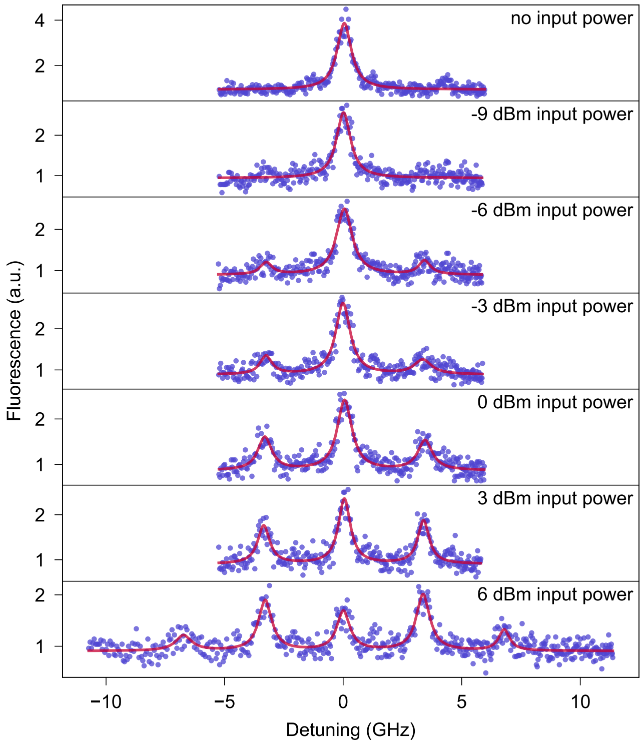


FIG. S7. Frequency modulation-induced sidebands of the SiV C-transition at zero magnetic field with varying acoustic powers.

resulting in the energies

$$E_{\pm} = \alpha \pm \sqrt{\left(\frac{\lambda_{\mathrm{SO}}}{2}\right)^2 + \beta^2 + \gamma^2}. \tag{S13}$$

The instantaneous quantities $\alpha, \beta, \gamma$ are given by the sum of a static term like $\alpha_0$ arising from pre-strain, and a time-dependent term like $\widetilde{\alpha}\sin(\omega t)$ from the oscillating SAW drive. For the SiV used in our measurements, for which $\beta, \gamma \ll \lambda_{\mathrm{SO}}$, the instantaneous energy shift of the C-transition is given by

$$\Delta E_C = \alpha_e - \alpha_g. \tag{S14}$$

As this is linear in strain, the time-dependent part of the energy shift is independent of any existing pre-strain and is given by

$$\Delta E_C(t) = (\widetilde{\alpha}_e - \widetilde{\alpha}_g)\sin(\omega t). \tag{S15}$$

This energy shift induces virtual states that couple to the lower excited state, with relative quasi-energies given by integer multiples of the drive frequency,

$$\Delta E_{C,k} = k\omega \tag{S16}$$

and populations

$$P_k \propto \left| J_k\left(\frac{\widetilde{\alpha}_e - \widetilde{\alpha}_g}{\omega}\right)\right|^2 \tag{S17}$$

in which $J_k$ are Bessel functions of the first kind.

**SAW power estimation.** Assuming that the SiV is located at the focus of the Gaussian SAW beam, finite element simulation allows us to determine the value of $\Delta\widetilde{\alpha} = \widetilde{\alpha}_e - \widetilde{\alpha}_g$, for a given SAW power $P$, from the strain

tensor amplitude $\epsilon$. However, in our experiments, the power at the location of the SiV is lower than the input microwave power by an efficiency factor $\eta$. Therefore, the quantity $\Delta\widetilde{\alpha}$ for an input power $P_{\text{in}}$ is given by

$$\Delta\widetilde{\alpha} = \Delta\widetilde{\alpha}_{\text{sim}}\sqrt{\frac{\eta P_{\text{in}}}{P_{\text{sim}}}} \tag{S18}$$

where $\Delta\widetilde{\alpha}_{\text{sim}}, P_{\text{sim}}$ are the values obtained from simulation. By using this relation, we fit the observed relative fluorescence intensities to the populations $P_k$ for different input powers, while varying the parameter $\eta$. The measured and fitted relative fluorescence intensities are shown in Fig. S8. We determine that the SiV is oriented longitudinally with respect to the SAW propagation direction, and estimate $\eta = 3.4 \times 10^{-4}$. The various factors contributing to $\eta$ are discussed further in Section VIII.

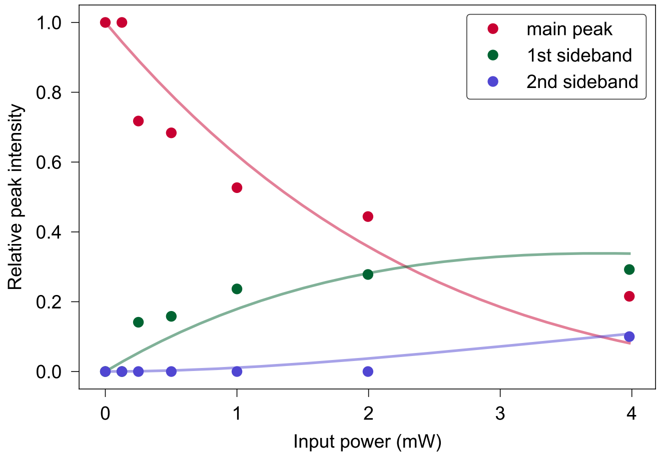


FIG. S8. Measured and fitted relative fluorescence intensities from Fig. S7, used for estimation of the power efficiency factor.

### B. $E_g$ strain response

Our calculations are performed in the basis of the eigenstates of the sum of the spin-orbit and axial Zeeman Hamiltonians, as we work in a non-zero magnetic field, in which we treat the strain and transverse magnetic field as perturbations. The initial Hamiltonian is given by

$$\begin{aligned}
\mathcal{H}_0 &= \mathcal{H}_{\text{SO}} + \mathcal{H}_{\text{Z}} && \text{(S19)}\\
&\approx -\frac{\lambda_{\text{SO}}}{2}\begin{bmatrix}0 & i\\ -i & 0\end{bmatrix} \otimes \begin{bmatrix}1 & 0\\ 0 & -1\end{bmatrix} + \frac{\gamma_S}{2}\mathcal{I}_2 \otimes \begin{bmatrix}B_Z & 0\\ 0 & -B_Z\end{bmatrix} && \text{(S20)}\\
&= \frac{1}{2}\begin{bmatrix}\gamma_S B_Z & 0 & -\lambda_{\text{SO}} i & 0\\ 0 & -\gamma_S B_Z & 0 & \lambda_{\text{SO}} i\\ \lambda_{\text{SO}} i & 0 & \gamma_S B_Z & 0\\ 0 & -\lambda_{\text{SO}} i & 0 & -\gamma_S B_Z\end{bmatrix} && \text{(S21)}
\end{aligned}$$

in which we have neglected the effect of the magnetic field on the orbitals, due to the small orbital quenching factor $q = 0.1$ [S5]. The eigenstates are given by $\{|e_{g+}\uparrow\rangle, |e_{g-}\downarrow\rangle, |e_{g-}\uparrow\rangle, |e_{g+}\downarrow\rangle\}$, in which $|e_{g\pm}\rangle = |e_{gX}\rangle \pm i\,|e_{gY}\rangle$, with energies given by $(\pm\lambda_{\text{SO}} \pm \gamma_S B_Z)/2$. The off-axis magnetic field term is

$$\mathcal{H}_{\text{Z,off}} = \frac{\gamma_S}{2}\mathcal{I}_2 \otimes \begin{bmatrix}0 & B_X - iB_Y\\ B_X + iB_Y & 0\end{bmatrix} \tag{S22}$$

which in the eigenstate basis is

$$\mathcal{H}_{\text{Z,off}} = \frac{\gamma_S}{2}\begin{bmatrix}0 & 0 & 0 & B_-\\ 0 & 0 & B_+ & 0\\ 0 & B_- & 0 & 0\\ B_+ & 0 & 0 & 0\end{bmatrix} \tag{S23}$$

in which $B_\pm = B_X \pm iB_Y$. This perturbs the eigenstates as

$$|e_{g+}\downarrow\rangle' \approx |e_{g+}\downarrow\rangle + \frac{\gamma_S B_+}{2\lambda_{\mathrm{SO}}} |e_{g+}\uparrow\rangle\,, \tag{S24}$$

$$|e_{g-}\uparrow\rangle' \approx |e_{g-}\uparrow\rangle + \frac{\gamma_S B_-}{2\lambda_{\mathrm{SO}}} |e_{g-}\downarrow\rangle\,. \tag{S25}$$

The strain term in the eigenstate basis is

$$\mathcal{H}_{\mathrm{st}} = \begin{bmatrix} \alpha & 0 & -\beta - i\gamma & 0 \\ 0 & \alpha & 0 & -\beta + i\gamma \\ -\beta + i\gamma & 0 & \alpha & 0 \\ 0 & -\beta - i\gamma & 0 & \alpha \end{bmatrix} \tag{S26}$$

which introduces a coupling between $|e_{g+}\downarrow\rangle$ and $|e_{g-}\uparrow\rangle$, given as

$$\Omega = \langle e_{g+}\downarrow' |\mathcal{H}_{\mathrm{st}}| e_{g-}\uparrow'\rangle \tag{S27}$$

$$= \frac{\gamma_S}{2\lambda_{\mathrm{SO}}} \left(B_-(-\beta - i\gamma) + B_-(-\beta - i\gamma)\right) \tag{S28}$$

$$= -\frac{\gamma_S(\beta + i\gamma)(B_X - iB_Y)}{\lambda_{\mathrm{SO}}} \tag{S29}$$

which is the generalized Rabi frequency when the oscillating strain field is resonant with the $|e_{g+}\downarrow\rangle \leftrightarrow |e_{g-}\uparrow\rangle$ transition, and the instantaneous quantities $\beta, \gamma$ are replaced by the amplitudes $\widetilde{\beta}, \widetilde{\gamma}$. The magnitude of $\Omega$ is equal to the measured Rabi frequency.

**SAW power estimation.** Similar to the case of the $A_{1g}$ strain response, the Rabi frequency for a given SAW power is estimated from simulation, and the measured Rabi frequencies are given by

$$\Omega = \Omega_{\mathrm{sim}} \sqrt{\frac{\eta P_{\mathrm{in}}}{P_{\mathrm{sim}}}}. \tag{S30}$$

The linear fit of $\Omega$ against $\sqrt{P_{\mathrm{in}}}$ (Fig. 4(a) in the main text) gives $\eta = 3.7 \times 10^{-5}$. This differs from the efficiency factor estimated from the $A_{1g}$ strain response by a factor of 9.2, and potential reasons for this discrepancy are discussed in Section VIII.

## VIII. SAW POWER EFFICIENCY

The power efficiency factors estimated from the $A_{1g}$ strain response and $E_g$ response (Rabi oscillations) are given by

$$\eta_{A_{1g}} = 3.4 \times 10^{-4}, \tag{S31}$$

$$\eta_{E_g} = 3.7 \times 10^{-5} \tag{S32}$$

as mentioned in Section VII. These factors can be expressed as a product of several individual efficiencies:

$$\eta_{A_{1g}} = \eta_{\mathrm{device}}, \tag{S33}$$

$$\eta_{E_g} = \eta_{\mathrm{device}} \times \eta_{\mathrm{magnetic}} \times \eta_{\text{pre-strain}}, \tag{S34}$$

$$\eta_{\mathrm{device}} = \eta_{\mathrm{input}} \times \eta_{\mathrm{propagation}} \times \eta_{\mathrm{alignment}}. \tag{S35}$$

The interpretation of each of these factors is explained below.

1. $\eta_{\mathrm{input}}$ is the conversion efficiency of the input microwaves to SAW by the transducer. It is estimated to be about $8.8 \times 10^{-2}$ from the electrical $S_{11}$ measurement (Fig. 2(b) in the main text).

2. $\eta_{\mathrm{propagation}}$ is due to the propagation losses of the SAWs travelling from the IDT to the SiV. Assuming that the conversion efficiencies for microwaves to SAW and SAW to microwaves are the same, this factor is estimated to be about $3.2 \times 10^{-1}$ which we infer from the electrical $S_{11}$ and $S_{21}$ measurements.

3. $\eta_{\text{alignment}}$ is due to the spatial misalignment between the SiV and the focus of the Gaussian SAW beam. Due to the large separation between the two IDTs in our device, it is not possible to determine the exact location of the focus during experiments, as both IDTs cannot be simultaneously imaged within one optical field of our confocal microscope. To identify the focal point, we first locate one IDT and then translate the optical field to where we expect the focus to be, after which we search for SiVs. It is possible to be misaligned by up to a few $\mu$m. The effect of this misalignment on the efficiency factor is shown in Fig. S9. Assuming a worst-case misalignment of 5 $\mu$m, this factor can be as low as $3.9 \times 10^{-3}$. In addition, misalignment along $y$ can also introduce $yy$, $xy$, and $zy$ components in the strain tensor, which changes the relations between $\Delta\alpha$, $\Omega$, and $P$. We do not attempt to evaluate these effects in detail.

4. $\eta_{\text{magnetic}}$. In our simulations, we assume that the magnetic field is oriented along the [001] direction. However, the direction of the magnetic field lines of a permanent magnet vary significantly depending on the spatial location. This introduces some uncertainty in the magnetic field components, which can vary the Rabi frequency.

5. $\eta_{\text{pre-strain}}$. The Rabi frequency from the $E_g$ strain response is significantly reduced by any existing pre-strain [S6]. However, the $A_{1g}$ strain response is robust against pre-strain. This factor accounts for the difference.

With the estimates for the efficiency factors mentioned above, $\eta_{\text{device}}$ varies between $2.8 \times 10^{-2}$ and $1.1 \times 10^{-4}$ depending on the misalignment. Therefore, the measured efficiency factor $\eta_{\text{device}} = 3.4 \times 10^{-4}$ is within reasonable limits. Additionally, $\eta_{E_g}/\eta_{A_{1g}} = \eta_{\text{magnetic}} \times \eta_{\text{pre-strain}} = 0.11$ indicates that $\eta_{A_{1g}}$ and $\eta_{E_g}$ are reasonably consistent, suggesting good agreement of our experimental results with the theory of the SiV strain response [S6], up to certain effects such as the precision of the magnetic field direction and uncontrollable pre-strain.

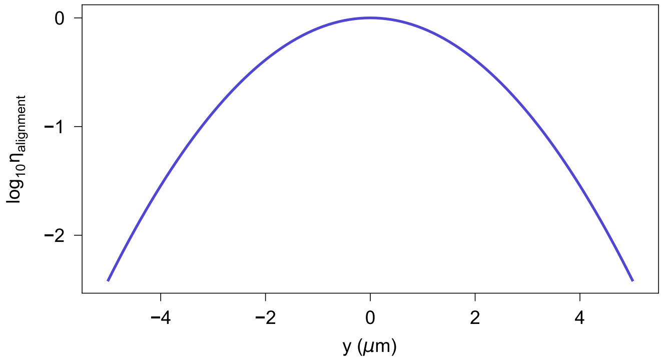


FIG. S9. Alignment efficiency factor as the location of the SiV is varied along the $y$-axis. The focus of the Gaussian SAW beam is at $y = 0$.


[S1] James F. Ziegler, M.D. Ziegler, and J.P. Biersack, "Srim-the stopping and range of ions in matter (2010)," Nuclear Instruments and Methods in Physics Research Section B: Beam Interactions with Materials and Atoms **268**, 1818 – 1823 (2010), 19th International Conference on Ion Beam Analysis.

[S2] Lu Zheng, Hui Dong, Xiaoyu Wu, Yen-Lin Huang, Wenbo Wang, Weida Wu, Zheng Wang, and Keji Lai, "Interferometric imaging of nonlocal electromechanical power transduction in ferroelectric domains," Proceedings of the National Academy of Sciences **115**, 5338–5342 (2018).

[S3] Lu Zheng, Di Wu, Xiaoyu Wu, and Keji Lai, "Visualization of Surface-Acoustic-Wave Potential by Transmission-Mode Microwave Impedance Microscopy," Physical Review Applied **9**, 061002 (2018).

[S4] Benjamin Pingault, David-Dominik Jarausch, Christian Hepp, Lina Klintberg, Jonas N. Becker, Matthew Markham, Christoph Becher, and Mete Atatüre, "Coherent control of the silicon-vacancy spin in diamond," Nature Communications **8**, 15579 (2017).

[S5] Christian Hepp, Tina Müller, Victor Waselowski, Jonas N. Becker, Benjamin Pingault, Hadwig Sternschulte, Doris Steinmüller-Nethl, Adam Gali, Jeronimo R. Maze, Mete Atatüre, and Christoph Becher, "Electronic Structure of the Silicon Vacancy Color Center in Diamond," Physical Review Letters **112**, 036405 (2014).

[S6] Srujan Meesala, Young-Ik Sohn, Benjamin Pingault, Linbo Shao, Haig A. Atikian, Jeffrey Holzgrafe, Mustafa Gündoğan, Camille Stavrakas, Alp Sipahigil, Cleaven Chia, Ruffin Evans, Michael J. Burek, Mian Zhang, Lue Wu, Jose L. Pacheco, John Abraham, Edward Bielejec, Mikhail D. Lukin, Mete Atatüre, and Marko Lončar, "Strain engineering of the silicon-vacancy center in diamond," Physical Review B **97**, 205444 (2018).
